# Supplementary material for: Phenomenology of a First Order Dark State Phase Transition
Source: arXiv:1803.08514 ancillary file (2018-03-22)
Supplement: Supplementary file 1 [file Documentation.pdf]

# Documentation for supplementary material

Dietrich Roscher,<sup>1,2</sup> Sebastian Diehl,<sup>1</sup> and Michael Buchhold<sup>3</sup>

<sup>1</sup>*Institut für Theoretische Physik, Universität zu Köln, D-50937 Cologne, Germany*

<sup>2</sup>*Department of Physics, Simon Fraser University, Burnaby, British Columbia, Canada V5A 1S6*

<sup>3</sup>*Department of Physics and Institute for Quantum Information and Matter,  
California Institute of Technology, Pasadena, CA 91125, USA*

(Dated: March 20, 2018)

We give detailed explanations for the interpretation of the animation files facilitated in this supplementary material. Additionally, some background information on the numerical methods and the derivation of the Langevin equation provided.

## I. KEY TO THE ANIMATED DATA

The renormalization flow of the deterministic potential  $V_k$  and in particular the noise kernel  $\chi_k$  can be quite dramatic. This is not always easily described in words or with individual, static pictures. We therefore provide some animated data of the renormalization group flow of decisive quantities for certain peculiar situations. In order to facilitate a proper interpretation, let us first consider the general representation of data in the animation files. With the exception of `PotZoom.avi`, which will be dealt with separately below, they are organized as in Fig. 1. In the following, we explain in detail how to interpret the data provided in the different panels.

*a. Configuration data (red dashed box)* This headline provides the initial values for the deterministic potential  $(\Delta, \mu, \lambda)$  and noise kernel  $(\kappa)$  used in computing the fRG evolution. Furthermore, spatial dimensionality  $d$  as well as the current value of the running RG scale  $k$  are given alongside.

*b. Evolving potential (1)* The first plot shows the evolution of the deterministic potential  $V_k(\nu)$ . Some rescaling of the vertical axis is performed to facilitate visibility of decisive features. The global minimum is marked by a red dot.

*c. Evolving noise kernel (2)* In the second graph, the evolution of the noise kernel  $\chi_k(\nu)$  is provided. Especially in the vicinity of first order phase transitions, strong rescaling of the vertical axis is performed in order to keep track of the immensely growing transient noise.

*d. Order parameter (3)* Here, the position of the global minimum of  $V_k$ ,  $\nu_0$ , is shown as a function of the RG scale  $k$  on a logarithmic scale. Since this is the order parameter of our phase transition, its value is of crucial importance.

*e. Convexity (4)* The last plot gives a rather abstract measure of the deterministic potential's curvature at the origin,  $V_k''(0)$ , and thus of convexity. Due to the shape of the initial potential and the property of suitably truncated fRG flows, this value is bound to be positive semidefinite in the beginning and end of the flow<sup>1</sup>. It

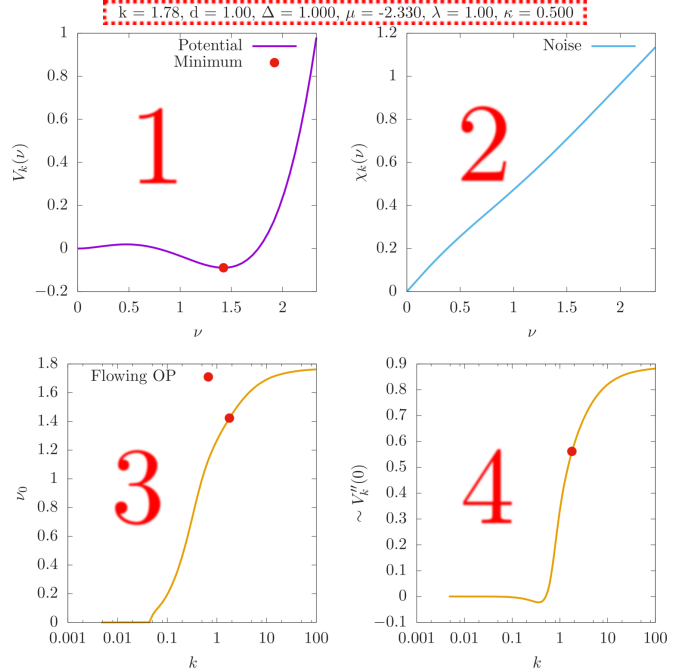

Figure 1. Prototypical screen shot of the animation files. Refer to main text for description of red marked sections

serves as a signature quantity for the order of the phase transition: continuous vanishing of the order parameter occurs only when  $V_k''(0) < 0$  for some  $k < k_{\text{barr}}$  even in the dark state phase in close vicinity of the transition. This change of curvature is synonymous to the removal of the potential barrier as discussed in the main paper.

## II. PHYSICAL INTERPRETATION

### A. Single configuration data

The four single configuration files organized in the scheme of Fig. 1 each correspond to a peculiar situation discussed in the main paper. In the following, we provide additional explanations for each file to enhance the viewing experience. The figures referred to here are found in the main paper.

<sup>1</sup> Note that inside the finite-density phase, convexity is approached only asymptotically, i.e.  $V_k''(0) < 0$  for all  $0 < k < k_{\text{barr}}$ .

- **d1S0Dis.avi** shows a configuration in the dark state phase close to a (second order) transition in one spatial dimension (Fig. 6). Special focus may be directed to the evolution of convexity of the effective potential and the ensuing continuous vanishing of the nontrivial minimum. The curvature achieves a negative value at  $k_{\text{barr}} \approx 0.5$ , where the non-trivial minimum is still finite. Thus, the potential barrier is removed before the fate of the minimum is settled and the transition becomes second order. The unspectacular and featureless flow of the noise kernel does not indicate any dominance of particular fluctuation configurations. Note that the continuous vanishing vs., for instance, the finite jump close to a first order transition is not to be confused with the physical continuity properties of the respective transitions. The RG parameter  $k$  is not a tuning parameter in a phase diagram. However, this behavior serves as an indication and provides useful insight on the nature of fluctuations, see also main paper.
- **d1S00r.avi** lies across the transition of **d1S0Dis.avi** inside the finite density phase (Fig. 8). At low scales, the noise kernel is suppressed for small but finite densities. This vanishing effectively extends the fluctuationless state space and stabilizes the non-trivial minimum of  $V_k$ . Note also that again at  $k_{\text{barr}} \approx 0.5$  the curvature of the potential turns negative, indicating the removal of the barrier.
- **d3F0Dis.avi** also represents a dark state configuration, but in three spatial dimensions and close to a first order phase transition (Fig. 10). The most significant finding here is the sudden change of the global minimum *in the presence* of the potential barrier at  $k \approx 5$ . The removal of the barrier is due to strong droplet-like fluctuations. This is indicated by a sharp double-peak structure of  $\chi_k$ , arising at a rather well-defined RG scale  $k_{\text{barr}} \approx 0.3$ . Since the global minimum of the potential is  $\nu_0 = 0$ , no finite density phase needs to be stabilized and a suppression of the noise kernel does not take place. Consequently, the double-peak structure of  $\chi_k$  survives down to the lowest scales. Note furthermore that the curvature of  $V_k$  is never rendered negative. This is equivalent to the finding of a discontinuously vanishing density and therefore solid evidence that the transition to be approached is of first order nature.
- **d3F00r.avi** again lies just across the transition of **d3F0Dis.avi** in the finite-density phase (Fig. 11). While the findings are naturally very similar to the latter at high and intermediate scales, droplet-like fluctuations prove insufficient to destroy the non-trivial minimum of  $V_k$  - the order parameter remains finite down to the lowest accessible scales.

The removal of the barrier, however, is again driven by an onset of massive droplet-like fluctuations at about  $k_{\text{barr}} \approx 0.3$ . Since the density remains finite, a suppression of the noise kernel takes place at the lowest scales. This is a numerically most challenging situation (see below) as  $\chi_k$  varies about several orders of magnitude within a very small range of densities  $\nu$ . For this reason, the flow could not be followed through to complete freeze-out as is the case for the other three configurations.

We believe that these configurations display the most important phenomena in a particularly clear way. However, the features exhibited are generic and can be found, more or less well-pronounced, across the whole phase diagram.

## B. Comparison of potentials

In the single configuration animation files, the evolution of the nontrivial minimums of  $V_k$  cannot be observed very well at low RG scales  $k$ . For sake of clarity, we did not consider it practical to change scales of the plot rapidly and massively to keep track with the depth of the respective minimum. Instead, **PotZoom.avi** provides a close-up view of all four deterministic potentials. Emergence of convexity and the destruction of the non-trivial minimum in the dark-state phase can be observed in detail here.

For comparison, the two configurations at each dimension are grouped together. Note that the global minimums may not be visible from the outset due to the scale of the plots. Once inside the field of vision, they are again marked with dots/diamonds.

The left panel represents the situation in  $d = 1$ . As long as the potential barrier is still present ( $k > k_{\text{barr}} \approx 0.5$ ), both configurations behave pretty similar. Only afterwards, the nontrivial minimum in the finite-density configuration slowly freezes to its infrared value, while the one in the dark state phase is continuously driven to zero.

The right panel displays the potentials in  $d = 3$  dimensions. Compared to  $d = 1$ , changes at scales  $k > 5$  are rather modest and so is the difference between the two configurations. Nevertheless, the nontrivial minimum of the dark state configuration attains a positive value at about  $k = 5$ . Only long afterwards, the potential barrier is removed.

While the final configurations in the left and right panels do not look very different qualitatively, their history certainly is and therefore allows to reliably discriminate between first and second order phase transitions.

## III. NUMERICAL IMPLEMENTATION

Last but not least, we give some details on the numerical implementation of the main flow equations (3.9a)

and (3.9b) in the paper or their extension with running wavefunction renormalization parameters or higher order noise kernels. Readers who are interested in the numerical solution of such field-dependent fRG equations may find it helpful to be pointed to possible pitfalls and our solutions for the scenario at hand.

We generally discretize the deterministic potential  $u_k$  and noise kernel  $\chi_k$  as a function of the density  $\nu$  on a uniform grid of 90-120 sites. The more pronounced the transient features of  $\chi_k$  are, the more sites are needed for a faithful representation. In particular, the vicinity of first order transitions, but also generally low initial noise levels call for a larger number of grid points. The  $k$ -integration of the flow equations is performed by a step-size controlled implicit Runge-Kutta algorithm of competing second and third order methods. From our experience, the enhanced stability properties of the implicit algorithms are generally better suited to the often stiff RG problems than the explicit ones. The inherently larger cost per integration step is usually more than compensated for by the larger step size available due to decreased error.

Derivatives of the potential and noise kernels are computed by different means, depending on the value of the running RG scale  $k$ . For larger  $k$ , a global basis spline fit is most suited to faithfully suppress numerical noise which tends to be amplified by the larger  $k^{d+1}$  factors in the flow equations. At lower  $k$ , it is more cost-efficient to trade this for (successive) spline interpolations with boundary conditions provided by analytical derivatives of higher order polynomial interpolation. Aside from being a rather fast and reliable method due to the possibility of employing efficient LAPACK eigenvalue solver routines, it is also most easily adapted to non-uniform grid configurations that become important during the course of the integration.

The most challenging problem in our scenario is the behavior of the noise kernel  $\chi_k$  when the droplet-indicating double-peak structure occurs. Since  $\chi_k(0) = 0$  is fixed, this can easily result into a values varying over several orders of magnitude across only a few grid points. Furthermore, the sharpness of the peak structure itself, while desirable for a physical interpretation, is not easily dealt with by the polynomial derivative operators. Due to these reasons, the initially uniform grid is not suited for such a situation anymore. Neither is it particularly helpful to utilize a fixed, but deformed grid, since the double-peak structure is not static and tends to move about the noise profile during the flow.

We therefore implemented a dynamically deformable grid. Whenever the local variation of the noise kernel exceeds a certain threshold value, an additional grid point is inserted. After smoothing the ensuing lattice and interpolation of  $u_k$  and  $\chi_k$ , the  $k$ -integration may be resumed. Likewise, points of particularly low variation are deleted, resulting in a self-contraction of the lattice in the most crucial regions. This alone is often not sufficient, as it usually leads to an accumulation of prohibitively

large numbers of lattice sites once the interesting feature begin to emerge. Therefore, we set a limit on the maximum number of grid points and reset the grid once it is reached. This is the reason for wiggly features sometimes observed in our figures of  $\chi_k$ . An ever larger number of grid points is able to progressively suppress these and also enlarge the accessible  $k$ -regime in the finite density phase across a first-order phase transition. This number may, however, become again prohibitively big and we therefore refrained from trying to remove each and every undesirable feature. After careful testing, we are confident that the latter do not influence the physical results beyond very minor quantitative variations anymore.

#### IV. ADIABATICALLY ELIMINATING $\sigma^{x,y}$

We outline here with more detail the adiabatic elimination of the spin operators  $\sigma^{x,y}$  in the Heisenberg Langevin equations. Their time evolution is fast compared to  $n_l$  due to their non-vanishing decay rate  $\sim \frac{\gamma}{2}$ . Thus they can be assumed to always remain in the steady state, i.e. adiabatically eliminated on time scales  $t > \gamma^{-1}$ . Setting  $\partial_t \sigma_l^{x,y} \stackrel{!}{=} 0$  in Eqs. (2.11), (2.12) in the main text yields

$$\xi_l^x = \mathcal{M}_{l,m} \sigma_m^x \Leftrightarrow \sigma_l^x = (\mathcal{M}^{-1})_{l,m} \xi_m^x, \text{ with} \quad (4.1)$$

$$\mathcal{M}_{l,m} = \frac{\gamma}{2} \delta_{l,m} + \Omega(\sigma_l^y (\Pi_m - 1) + \text{H.c.}) \delta_{m, \text{nn } l} + i0^+.$$

The operator  $\mathcal{M}$  represents an operator valued Green's function, i.e. describes the forward time evolution of the system for an infinitesimal time step  $\Delta t = 0^+$  and thus has to be interpreted as a retarded propagator  $\sim i0^+$ , and is therefore regular. It shows that  $\sigma_l^x$  is proportional to the noise  $\xi_l^x$ . Inserting Eq. (4.1) into the equation of motion for  $\sigma_l^y$  leads to

$$\begin{aligned} \frac{\gamma}{2} \sigma_l^y &= \xi_l^y - 2\Omega \Pi_l (2n_l - 1) \\ &+ \Omega \left[ \sum_{j \text{ nn } l} (\Pi_j - 1) (\mathcal{M}^{-1})_{j,s} \xi_s^x \xi_m^x (\mathcal{M}^{-1})_{m,l} \right]. \end{aligned} \quad (4.2)$$

We perform an expansion of the inverse of  $\mathcal{M}$  in terms of nearest neighbor couplings  $\mathcal{T}$ , i.e.  $\mathcal{M}^{-1} = (\gamma/2 + \mathcal{T})^{-1} = 2/\gamma - 4/\gamma^2 \mathcal{T} + o(\mathcal{T}^2)$ . Due to the sum over nearest neighbors and the locality of the noise kernel, the diagonal elements of  $\mathcal{M}^{-1}$  do not contribute and the leading order contribution in this expansion is  $\sim \mathcal{T}$ . Higher order contributions in the nearest neighbor coupling are suppressed by  $\gamma$  and less relevant. This yields

$$\sigma_l^y = (\mathcal{K}^{-1})_{j,l} (\xi_l^y - 2\Omega \Pi_l (2n_l - 1)), \quad (4.3)$$

The final Heisenberg-Langevin equation for the density variable is obtained by inserting the solution for  $\sigma_l^y$  into Eq. (2.10). This yields Eq. (2.14) with  $\mathcal{K}$  defined in Eq. (2.15).
